# Supplementary material for: Integrating genealogical and dynamical modelling to infer escape and reversion rates in HIV epitopes
Source: arXiv:1302.1098 ancillary file (2013-02-11)
Supplement: Supplementary file 1 [file supplementary.pdf]

# Integrating genealogical and dynamical modelling to infer escape and reversion rates in HIV epitopes: Supplementary Material

Duncan Palmer[1,*], John Frater[2,3], Rodney Philips[2,3], Angela McLean[3,4], Gil McVean[1]

**1 Department of Statistics, 2 Nuffield Department of Clinical Medicine, 3 The James Martin 21st Century School, Peter Medawar Building for Pathogen Research, 4 Department of Zoology, South Parks Road, University of Oxford, Oxford, United Kingdom**

∗ **E-mail: duncan.palmer@stats.ox.ac.uk**

## S1 Justification of combining tree pruning and BEAST

To create the sequences observed at the tips of the true genealogy together with the HLA and escape status of the host, three processes occur concurrently. We have a collection of epidemiological parameters $\Psi$ which govern the structure of true underlying genealogy $G$, mutation parameters $\Theta$ which determine the distribution of sequences at the tips (excluding the epitope of interest), and finally some escape parameters $\boldsymbol{\lambda}$ governing the distribution of presence of escape and HLA type of the host at the tips. Suppose we have the following collection of priors and observed data:

- Priors $f$, $g$, $h$ on $\Psi$, $\Theta$ and $\boldsymbol{\lambda}$ respectively.
- Observed sequences at the tips $X$ (excluding epitope) and observed presence or lack of escape at the tips and HLA information, $E$.

We wish to determine

$$P(\boldsymbol{\lambda}|X, E, f, g, h). \tag{1}$$

BEAST provides samples from $P(G, \Theta, \Psi|X, f, g)$. To sample from $P(\boldsymbol{\lambda}|X, E, f, g, h)$, we marginalise over $G$, $\Theta$ and $\Psi$ in $P(\boldsymbol{\lambda}, G, \Theta, \Psi|X, E, f, g, h)$ by considering:

$$P(\boldsymbol{\lambda}, G, \Theta, \Psi|X, E, f, g, h) = P(G, \Theta, \Psi|X, E, f, g, h)\; P(\boldsymbol{\lambda}|X, E, f, g, h, G, \Theta, \Psi) \tag{2}$$

$$= \frac{P(G, \Theta, \Psi|X, E, f, g, h)}{P(G, \Theta, \Psi|X, f, g, h)}\; P(G, \Theta, \Psi|X, f, g, h)\; P(\boldsymbol{\lambda}|E, h, G). \tag{3}$$

If we assume that

$$\frac{P(G,\Theta,\Psi|X,E,f,g,h)}{P(G,\Theta,\Psi|X,f,g,h)} \approx 1 \tag{4}$$

then,

$$P(\boldsymbol{\lambda},G,\Theta,\Psi|X,E,f,g,h) \approx P(G,\Theta,\Psi|X,f,g,h)\; P(\boldsymbol{\lambda}|E,h,G). \tag{5}$$

Note that this statement is equivalent to assuming that escape within the epitope of interest does not have any impact on our inference of the underlying tree. The neutral mutation parameters or parameters governing the evolution of the number of infecteds in the epidemic. By sampling from $P(G,\Theta,\Psi|X,f,g)$ (the output from BEAST), and further sampling $P(\boldsymbol{\lambda}|E,h,G)$ from these BEAST samples, we are averaging $P(\boldsymbol{\lambda},G,\Theta,\Psi|X,E,f,g,h)$ over $G,\Theta,\Psi$ and thus sampling from the desired distribution $P(\boldsymbol{\lambda}|X,E,f,g,h)$.

## S2 Rewriting the sampled reconstructed process as a generalised pure birth process

In Nee et al. [1], it is shown that a birth-death process with complete sampling at the present can be rewritten as a generalised birth process with variable rate $\lambda P(t,T)$. In a similar manner, we show that the inclusion of sampling a proportion $\rho$ of the extant lineages at the present can also be rewritten as a pure birth process. This, though not explicitly stated, is what was done between equations 2 and 3 in Yang and Rannala [2].

Using a Dirac delta function at the present in order to include a mass extinction of $(1-\rho)$ of the population which is equivalent to sampling a proportion $\rho$ at the present, Nee et al. [1] consider a generalised birth-death process with constant birth rate $\lambda$ and death rate $\mu(t,T) = \mu - \delta(t,T)\log(\rho)$. Using Kendall's derivations [3], under this new process $1 - p_0(t) = 1 - \xi_t$ and

$$P_s(t,T) = \frac{\rho(\lambda-\mu)}{\rho\lambda + (\lambda(1-\rho)-\mu)\exp(-(\lambda-\mu)(T-t))}, \tag{6}$$

where the subscripted $s$ denotes sampling. Consider a pure birth process with speciation rate $\lambda P_s(t,T)$. Using Kendall's notation [3], the probability of $i$ lineages existing at time $t$ (by the process being pure

birth we have effectively conditioned on the lineages surviving to the present, time $T$) is

$$\hat{p_i}(t) = (1-\eta_{t,T})\eta_{t,T}^{i-1} \quad i > 0, \tag{7}$$

$$\text{where} \quad \eta_{t,T} = \frac{\lambda\rho(1-\exp(-(\lambda-\mu)t))}{\lambda\rho - (\mu - \lambda(1-\rho))\exp(-(\lambda-\mu)T)}. \tag{8}$$

It can then be checked that $\eta_{t,T} = u_t P_s(0,T)/P(0,t)$ to show that this is the same as considering a full process with births and deaths, sampling and reconstructing the transmission history.

Applying the same steps as in Nee et al. [1], the probability that a birth-death process surviving to $t$ with $i$ descendants survives to time $T$ is

$$z_i := \frac{(1-u_t)u_t^{i-1}(1-(1-P_s(t,T))^i)}{\sum_{j=1}^{\infty}(1-u_t)u_t^{j-1}(1-(1-P_s(t,T))^j)} \tag{9}$$

$$= \frac{P(0,t)}{P_s(0,T)}(1-u_t)u_t^{i-1}(1-(1-P_s(t,T))^i). \tag{10}$$

Now create the reconstructed process with sampling. Of $k$ lineages existing in the past, at time $t$, we require those ancestries which result in $i$ lineages at the present, time $T$.

$$\sum_{k=i}^{\infty} \frac{z_k \binom{k}{i} \left(P_s(t,T)\right)^i \left(1-P_s(t,T)\right)^{k-i}}{1-(1-P_s(t,T))^k}. \tag{11}$$

This simplifies to

$$\left(1 - u_t\frac{P_s(0,T)}{P(0,t)}\right)\left(u_t\frac{P_s(0,T)}{P(0,t)}\right)^{i-1}, \tag{12}$$

as required. Using the birth-death process with Dirac delta function described above, it can be derived that the probability a lineage at time $t$ leaves exactly one descendant is

$$p_1(t) := \frac{P_s(t,T)\,(\lambda-\mu)}{\lambda(1-\rho) - \mu + \lambda\rho\exp((\lambda-\mu)(T-t))} \tag{13}$$

$$= \frac{1}{\rho}\exp(-(\lambda-\mu)(T-t))(P_s(t,T))^2, \tag{14}$$

as stated in Yang and Rannala [2] (this is simply $P_s(t,T)\,(1-\eta_{T-t,T-t})$). Using exactly the same arguments as above, the joint distribution of node times (measured backwards from the present), conditional

on survival, $n$ tips, a root time $t_1$ ago and sampling at rate $\rho$ can be written as

$$f(\mathbf{s}|n, t_1, \lambda, \mu, \rho, \text{survival}) = (n-2)! \prod_{j=2}^{n-1} \lambda \frac{p_1(t_j)}{\nu_{t_1}}, \tag{15}$$

$$\text{where} \quad \nu_t = 1 - \frac{1}{\rho} P_s(0,t) \exp(-(\lambda-\mu)t). \tag{16}$$

To make this more clear, the two lineages from the initial split make it into the sample with single progeny (themselves), the probability that this occurs is $p_1(t_1)^2$. Births of new lineages occur at rate $n(t)\lambda P_s(t,T)$, and the probability of each leaving exactly 1 sampled descendant is $p_1(t)$. In order to condition on $n$ individuals in the sample, and root time $t_1$, we must make sure that from the two initial lineages there are $n$ descendants, this amounts to division by

$$(n-1)\left(P_s(0,t)\left(1-\eta_{T-t_1,T-t_1}\right)\right)^2 \eta_{T-t_1,T-t_1}^{n-2} \tag{17}$$

$$= (n-1)\left(P_s(0,t)\left(1-\frac{u_t P_s(0,T)}{P(0,T)}\right)\right)^2 \left(\frac{u_t P_s(0,T)}{P(0,T)}\right)^{n-2} \tag{18}$$

$$= (n-1)p_1(t)^2\left(1-\frac{p_1(t)}{P_s(0,t)}\right)^{n-2}. \tag{19}$$

Finally unseen transmissions. These events along a given lineage occur independently of seen events and thus may be placed independently at rate $\lambda p_0(t)$. This observation means that we may lay unseen transmission events over a variable pure birth tree.

## S3 Detailed Methods

**Data**: The Swiss-Spanish intermittent treatment trial (SSITT) was a study of structured treatment interruptions in chronically HIV-infected patients, described in detail elsewhere [4]. A single sequence (from population sequencing) from each of the individuals is sampled at a single time-point [5]. We consider the HLA typed subset of the cohort for our analyses, and remove sequences in which $> 10\%$ of nucleotides could not be called. As not all patients were sequenced in each gene this led to a collection of 79, 67, and 53 HLA typed sequences for gag, pol and nef respectively.

**Definition of escape mutation**: All amino acid changes at the same point(s) as a previously defined and escape mutations validated *in vitro* are considered to confer escape. This is clearly an imperfect definition, but provides a sensible compromise between the clear overestimation of allowing all mutations

within an epitope to be defined as escape, and only considering mutations validated as escapes by *in vitro* assays.

**Reference sequences**: For the later tree pruning step in our method, sequences sampled over a collection of dates are required to estimate the molecular clock rate. This is used to convert between units of time (from "calendar time" (measured in *years*), to generation time (measured in units of $2N$ generations)), and is needed to obtain our rate estimates for $\lambda_{\text{esc}}$ and $\lambda_{\text{rev}}$ in $years^{-1}$. We added dated European B clade sequences with full gene coverage before the year 2000 from the Los Alamos HIV sequence database [6]. These consisted of 52, 14 and 68 gag, pol and nef sequences respectively.

**Alignment**: We use HIValign [7] which uses a hidden Markov model (HMM) to align viral sequence data, followed by manual editing of the resulting alignment.

**Data trimming**: Non-B clade sequences were identified using recombinant identification program (RIP) [8] and were removed if confirmed as non-B clade or could not be identified at the 90% significance level. The epitope under investigation was removed from the alignment, as this is considered to be under selection, and could therefore lead to clustering of escape mutations and thus affect rate estimates. We do not remove all epitopes under selection as this would involve removing the majority of our sequence information. This led to 58, 57 and 50 gag, pol and nef sequences.

**Nucleotide substitution model**: We used jmodeltest [9] Akaike information criterion (AIC) scores to determine the nucleotide substitution model to use. We found that the generalised time-reversible model with a gamma distributed substitution rate across sites and a proportion of invariant sites ($GTR+\Gamma+I$) was chosen for each gene.

**Sampling from the posterior tree distribution**: We ran BEAST [10] on our stripped sequence data, $X$, to generate samples from the posterior distribution of trees given an exponential coalescent tree prior, together with the $GTR+\Gamma+I$ model of nucleotide substitution. We did not use a model which considers codon position as we found that this significantly reduced estimated sample sizes (ESS). Chains are 100,000,000 updates long.

**Tree pruning**: After sampling a genealogy from the posterior output by BEAST, we use extra information, $E$, in order to determine estimates of ($\lambda_{\text{esc}}$, $\lambda_{\text{rev}}$). Our algorithm is based on that first proposed in [11], replacing the four nucleotide state space $\mathcal{N} := \{A, C, G, T\}$ with $\mathcal{S} := \{(0,0),(0,1),(1,0),(1,1)\}$. We denote the pair $(a, b)$; $a, b \in \{0, 1\}$ such that $\{0, 1\}$ in the first entry denotes {HLA mismatch, HLA match}, and $\{0, 1\}$ in the second entry denotes {no escape mutation, escape mutation}. Transmission

is assumed to take place at rate $\lambda$ and the probability that a given individual is HLA matched at the epitope under investigation is $p$. We assume $p$ is constant in the population over time, as any selection on hosts would occur on far larger timescales [12]. We may then obtain the probability of a given configuration of the data $E$ at the tips, conditional on the genealogy $G$ and a collection of parameters $\boldsymbol{\lambda} = \{\lambda, \lambda_{\text{esc}}, \lambda_{\text{rev}}, p\}$, which model escape and reversion down each lineage governed by an instantaneous rate matrix $\mathbf{Q}$ which we specify. As in [13], we suppose that escape may only occur from the $(1,0)$ state at rate $\lambda_{\text{esc}}$ and reversion may only occur from the $(0,1)$ state at rate $\lambda_{\text{rev}}$ (Figure 1$a$). Thus, the instantaneous rate matrix $\mathbf{Q}$ may be defined

$$\mathbf{Q} = \begin{array}{c} \\ (0,0) \\ (0,1) \\ (1,0) \\ (1,1) \end{array} \begin{array}{c} \begin{array}{cccc} (0,0) & (0,1) & (1,0) & (1,1) \end{array} \\ \begin{pmatrix} -\hat{\lambda}(t)p & 0 & \hat{\lambda}(t)p & 0 \\ \lambda_{\text{rev}} & -\lambda_{\text{rev}} - \hat{\lambda}(t)p & 0 & \hat{\lambda}(t)p \\ \hat{\lambda}(t)(1-p) & 0 & -\lambda_{\text{esc}} - \hat{\lambda}(t)(1-p) & \lambda_{\text{esc}} \\ 0 & \hat{\lambda}(t)(1-p) & 0 & -\hat{\lambda}(t)(1-p) \end{pmatrix} \end{array}, \tag{20}$$

where $\hat{\lambda}(t) = \lambda p_0(T_{\text{MRCA}} - t)$, with time increasing towards the present. $T_{\text{MRCA}}$ is the time before the present of the most recent common ancestor (MRCA), when $t = 0$. We use the convention that $Q_{ij}$ refers to the transition from state $i$ to state $j$. $p_0(t)$ is the probability that a lineage at time $t$ in the past does not have any sampled descendants.

$$p_0(t) = 1 - \frac{\rho(\lambda - \mu)}{\rho\lambda + (\lambda(1-\rho) - \mu)\exp(-(\lambda - \mu)t)}, \tag{21}$$

where $\mu$ is the rate of becoming non-infectious, and $\rho$ is the sampled proportion at the present which we estimate separately [2]. This extra factor must be included to avoid double counting of transmission events, as we assume transmission events occur at coalescences within the tree. Indeed, these internal nodes are precisely those transmission events which result in a descendant which is sampled at the present, $1 - p_0(T - t)$. $p_0(t)$ for a sampled birth-death process was originally derived in [2] and details of the derivation, excluded from the original paper, are given in the supplementary text S3. We wish to determine the probability of a branch beginning in state $i$ and ending in state $j$ in order to then evaluate the likelihood over the entire tree. The time dependency in $\hat{\lambda}(t)$ means that this no longer has a simple closed

form (as is the case for constant coefficients). If we define $\mathbf{P}(t) = (P_{(0,0)}(t), P_{(0,1)}(t), P_{(1,0)}(t), P_{(1,1)}(t))$ to be the vector of probabilities of observing each state in $\mathcal{S}$ at time $t$, we must numerically evaluate the solution to

$$\dot{\mathbf{P}}(t) = \mathbf{P}(t)\mathbf{Q}(t) \tag{22}$$

at the end of each branch within the tree, $\mathbf{P}(t_i)$ where $t_i$ is the time of node $i$, subject to the initial condition $\mathbf{P}(t_k)$ being one of the four states with certainty at the start of the branch, where node $k$ is the parent of node $i$. This amounts to evaluating the probability of starting in any one of the four states and ending in any one of the four states for each branch within the tree, which we define as $P_{s_k s_j}$ for $s_k, s_j \in \mathcal{S}$. The assumption of exactly one transmission at each internal node requires an alteration to the original pruning algorithm. We make the following change: pick with equal probability the branch which exists as a result of the transmission (as we are using the phylogeny as a proxy for the transmission tree, and assume that exactly one transmission takes place immediately after each internal node), the other branch represents virus remaining in the transmitting host. As we assume this transmission has taken place at the internal node, no change in the escape state can occur. We therefore sum over the two HLA states, keeping the escape state fixed at node $k$. Adopting the notation in [11], let $s_k \in \mathcal{S}$ denote the state of the individual at node $k$. To incorporate the sum over HLA types, we include the following additional notation: define $s_{k_{\text{HLA}}}$ as the state with the same escape state as node $k$, and first entry HLA. That is, $s_{k_{\text{HLA}}} := (\text{HLA}, s_k(2))$ where $\text{HLA} \in \{0, 1\}$. We may now write our process in terms of conditional likelihoods. $L_s(k)$ is defined as the likelihood of the data below node $k$ conditional on it having state $s$. Node $k$ has daughter nodes $i$ and $j$,

$$\begin{aligned} L_{s_k}(k) = &\frac{1}{2}\left(\left(\sum_{s_i \in \mathcal{S}} \left((1-p)P_{s_{k_0} s_i}(t_i) + pP_{s_{k_1} s_i}(t_i)\right) L_{s_i}(i)\right)\left(\sum_{s_j \in \mathcal{S}} P_{s_k s_j}(t_j) L_{s_j}(j)\right)\right. \\ &\left. + \left(\sum_{s_i \in \mathcal{S}} P_{s_k s_i}(t_i) L_{s_i}(i)\right)\left(\sum_{s_j \in \mathcal{S}} \left((1-p)P_{s_{k_0} s_j}(t_j) + pP_{s_{k_1} s_j}(t_j)\right) L_{s_j}(j)\right)\right). \end{aligned} \tag{23}$$

Finally considering the prior distribution at the root node (defined as node 0, with distribution of states $\pi_{s_0}$),

$$L = \sum_{s_0 \in \mathcal{S}} \pi_{s_0} L_{s_0}(0). \tag{24}$$

Assuming the initial state $s_0$ will not display the escape mutation and have the restricting HLA allele with probability $p$, $\pi_{s_0} = (1-p, 0, p, 0)$. Part of the output of BEAST is used to determine parameters in the pruning algorithm. Under the exponential coalescent prior, $\lambda$ is equal to $g + \mu$ where $g$ is the exponential growth rate of the infected population sampled in the MCMC [14]. $\mu$ is the estimated rate of becoming non-infectious, which we set at 0.1 $years^{-1}$ [13,15], this emerges as the coalescence rate scales with the total infected number of individuals [14]. $p$ is estimated from data in the HLA FactsBook [16]. Code to evaluate the likelihood of a genealogy conditional on some parameter set and tip data was coded in C++ using boost libraries and the odeint package [17], and checked against R code.

**Integrating over trees**: We assume HLA and escape information is uninformative about the tree topology (see supplementary text S1). From the BEAST output sample from the posterior, we subsample 1000 trees. *A priori* it is unknown where the majority of probability mass of $P(\boldsymbol{\lambda}|E, h, G)$ lies (where $h$ is our prior on $\boldsymbol{\lambda}$), so we perform simple hill climbing to determine its maximum, $P_G^{\max}$. We may then approximate the surface by a bivariate normal distribution. Next we define a 99.9% error ellipse based on this approximation within which to evaluate $P(\boldsymbol{\lambda}|E, h, G)$ for each genealogy $G$, choosing the smallest $50 \times 50$ lattice containing the error ellipse and enforce a $U[10^{-20}, 10^3]$ prior on $\lambda_{\text{esc}}$ and $\lambda_{\text{rev}}$. To ensure that the normal approximation encompasses the majority of the mass, we check $P(\boldsymbol{\lambda}|E, h, G)$ on the error ellipse and evaluate over the entirety of $[10^{-20}, 10^3] \times [10^{-20}, 10^3]$ if at any point it lies above the threshold of $P_G^{\max}/1000$. We then normalise these probability densities over the domain on which they are evaluated. In order to integrate over trees, we must define a common lattice over which to sum. This is achieved by defining an $800 \times 800$ grid on the minimum region of parameter space which encloses the union of domains defined for each probability density. We interpolate each surface, before summing over all surfaces obtained. The normalisation of this marginalisation defines our estimate of $P(\boldsymbol{\lambda}|X, E, f, g, h)$, where $f$ and $g$ are priors on epidemiological parameters and substitution parameters respectively (see supplementary text S1 for full details).

**Credible regions**: These are defined in $P(\boldsymbol{\lambda}|X, E, f, g, h)$ by determining the contour level enclosing $\alpha$% of the probability mass, where $\alpha$ is the percentage credible region required.

**Mahalanobis distance**: The distance of a vector $x = (x_1, x_2, \ldots, x_n)$ from a group of values with mean $\eta = (\eta_1, \eta_2, \ldots, \eta_n)$ and covariance matrix $\Sigma$ is $D(x) = \sqrt{(x-\eta)\Sigma^{-1}(x-\eta)^T}$ [18].

## S4 Equivalence of ODE model and composite likelihood

The ODE system of [13] may be written as $\dot{Y} = \tilde{Q}Y$ where $\tilde{Q} = Q + D$, $D$ the diagonal matrix with $D_{ii} = \lambda - \mu$, $D_{ij} = 0$; $i \neq j$, and $Y$ is the number of infected individuals in each class. The general solution of $\dot{X} = AX$, where $A$ has constant entries is $X = \sum_{i=1}^{n} c_j \nu_j e^{\omega_i t}$ where $\nu_i$ and $\omega_i$ are the eigenvectors and corresponding eigenvalues of $Q$.

$$Q\nu = \omega\nu \quad \Rightarrow \quad (Q + D)\nu = \omega\nu + D\nu. \tag{25}$$

$D$ diagonal $\Rightarrow$ $(Q + D)\nu = (\omega + \lambda - \mu)\nu$. Therefore, solutions of $\dot{Y} = \tilde{Q}Y$ may be written as $Y = e^{(\lambda-\mu)t}P$ where $P$ is the solution to $\dot{P} = QP$. $P$ is simply a rescaling of $Y$ by total population size through time. Therefore, using the ODE approach is equivalent to assuming a multinomial distribution over the four possible states, subject to some initial condition. Thus, we may consider the likelihood of the parameters data under the ODE model as a composite likelihood $L_c(\boldsymbol{\lambda}|E) = (1-p)\left(\prod_{j=1}^{m} P_{(0,0)s_j}(T)\right) + p\left(\prod_{j=1}^{m} P_{(1,0)s_j}(T)\right)$, where $m$ is the total number of cross-sectional samples. Note the implicit assumption that $\lambda$ is not a function of time, hence the ODE model is equivalent to the assumption that all transmission events are unseen ($\rho = 0$), and therefore the genealogy is completely star-like and all lineages are independent, with the same initial condition.

## S5 Justification of validity of hypothesis testing

In order to test simple hypotheses, we need to compute the likelihood under the various models, and perform a likelihood ratio test. To do this, we make the following observation:

First, let $\Psi_{\boldsymbol{\lambda}} := \Psi \setminus \boldsymbol{\lambda}$ and note $P(E|G,\Theta,\Psi) = P(E|G,\Psi)$. Then,

$$L(\boldsymbol{\lambda} = \boldsymbol{\lambda}^*|X,E) \propto \int_G \int_{\Psi_{\boldsymbol{\lambda}}} \int_{\Theta} P(X,E|G,\Theta,\Psi_{\boldsymbol{\lambda}},\boldsymbol{\lambda}^*)P(G,\Theta,\Psi_{\boldsymbol{\lambda}},\boldsymbol{\lambda}^*)\ dGd\Psi_{\boldsymbol{\lambda}}d\Theta \tag{26}$$

$$\Rightarrow \quad L(\boldsymbol{\lambda} = \boldsymbol{\lambda}^*|X,E) = C \int_G \int_{\Psi_{\boldsymbol{\lambda}}} \int_{\Theta} P(X,E|G,\Theta,\Psi_{\boldsymbol{\lambda}},\boldsymbol{\lambda}^*)P(G,\Theta,\Psi_{\boldsymbol{\lambda}},\boldsymbol{\lambda}^*)\ dGd\Psi_{\boldsymbol{\lambda}}d\Theta \tag{27}$$

$$= \widetilde{C} \int_G \int_{\Psi_{\boldsymbol{\lambda}}} \int_{\Theta} \frac{P(X|G,\Theta,\Psi_{\boldsymbol{\lambda}},\boldsymbol{\lambda}^*)P(G,\Theta,\Psi_{\boldsymbol{\lambda}},\boldsymbol{\lambda}^*)}{P(X)} P(E|G,\Psi_{\boldsymbol{\lambda}},\boldsymbol{\lambda}^*)\ d\Theta d\Psi_{\boldsymbol{\lambda}}dG \tag{28}$$

$$= \widetilde{C} \int_G \int_{\Psi_{\boldsymbol{\lambda}}} \int_{\Theta} P(G,\Theta,\Psi_{\boldsymbol{\lambda}},\boldsymbol{\lambda}^*|X)P(E|G,\Psi_{\boldsymbol{\lambda}},\boldsymbol{\lambda}^*)\ d\Theta d\Psi_{\boldsymbol{\lambda}}dG \tag{29}$$

$$= \widetilde{C} \int_G \int_{\Psi_{\boldsymbol{\lambda}}} \int_{\Theta} P(G,\Theta,\Psi_{\boldsymbol{\lambda}}|X)P(E|G,\Psi_{\boldsymbol{\lambda}},\boldsymbol{\lambda}^*)\ d\Theta d\Psi_{\boldsymbol{\lambda}}dG \tag{30}$$

$$\approx \frac{1}{N}\sum_{i=1}^{N} P(E|\boldsymbol{\lambda},G_i,\Psi_{\boldsymbol{\lambda},i}) \qquad G_i,\Psi_{\boldsymbol{\lambda},i} \sim P(G,\Theta,\Psi_{\boldsymbol{\lambda}}|X). \tag{31}$$

Thus, by sampling from BEAST and computing the mean of the probability of observing $E$ under the parameters conditional on the genealogy and epidemiological parameters, we approximate the likelihood.

## S6 Connections between formulations of reconstructed tree likelihoods

For what follows, we need the following probabilities, derived by Kendall [3]:

$$P(\tilde{t},t) = \frac{\lambda-\mu}{\lambda-\mu\exp(-(\lambda-\mu)(t-\tilde{t}))}, \tag{32}$$

$$p_0(t) = 1 - P(0,t), \tag{33}$$

$$p_i(t) = P(0,t)(1-u_t)u_t^{i-1} \quad i>0, \tag{34}$$

where

$$u_t = \frac{\lambda(1-\exp(-(\lambda-\mu)t))}{\lambda-\mu\exp(-(\lambda-\mu)t)}. \tag{35}$$

$P(\tilde{t},t)$ is the probability that a single lineage alive at time $\tilde{t}$, has at least one descendant at the later time $t$, $p_0(t)$ is the probability that a lineage starting at time 0 has no descendants, some time $t$ later. Finally $p_i(t)$ is the probability that a lineage starting at time 0 has $i$ descendants after time $t$.

In [19], the likelihood of a reconstructed birth-death tree with speciation times $\mathbf{s} = \{s_1, s_2, \ldots, s_{n-2}\}$ (where $s_i$ is the $i^{\text{th}}$ speciation event measured and indexed backwards in time), $n$ leaves, and some

labelled history $F$, given a transmission rate $\lambda$, a death rate $\mu$ and time of the first transmission event in the tree (the root), $s_{n-1} := t$ is derived as

$$f_{\text{Thompson}} := f(\mathbf{s}, n, F|\lambda, \mu, t) = \frac{2^{n-1}}{n!}\lambda^{n-2}(p_1(t))^2 \prod_{j=1}^{n-2} p_1(s_j). \tag{36}$$

If we condition on survival of the tree and labellings, then we can obtain the likelihood in [1], $f_{\text{Nee}}$. Conditioning on survival amounts to dividing by the probability that the two lineages at the root survive to the present, $P(0,t)^2 = (1 - p_0(t))^2$. The number of possible labellings is $|F| = 2^{n-1}/(n!(n-1)!)$. Therefore,

$$\begin{aligned}
f_{\text{Nee}} :&= f(\mathbf{s}, n|F, \lambda, \mu, t, \text{survival}) &(37)\\
&= \frac{f_{\text{Thompson}}}{|F|P(0,t)^2} &(38)\\
&= \frac{n!(n-1)!}{2^{n-1}(1-p_0(t))^2}\left(\frac{2^{n-1}}{n!}\lambda^{n-2}(p_1(t))^2\prod_{j=1}^{n-2}p_1(s_j)\right) &(39)\\
&= \frac{(n-1)!}{P(0,t)^2}\left(\lambda^{n-2}((1-u_t)P(0,t))^2\prod_{j=1}^{n-2}p_1(s_j)\right) &(40)\\
&= (n-1)!\lambda^{n-2}(1-u_t)^2\prod_{j=1}^{n-2}p_1(s_j). &(41)
\end{aligned}$$

Rewritten, with time increasing forwards and the present set at time $T$, 0 the time of the initial infected individual, and $t_i$ the time of the $(i-1)^{\text{th}}$ speciation event, indexed forwards through time,

$$\begin{aligned}
f_{\text{Nee}} &= (n-1)!\lambda^{n-2}(1-u_t)^2\prod_{j=1}^{n-2}p_1(s_j) &(42)\\
&= (n-1)!\lambda^{n-2}(1-u_{(T-t_2)})^2\prod_{j=3}^{n}(1-u_{(T-t_j)})P(t_j,T). &(43)
\end{aligned}$$

This is the likelihood in equation 20 of [1]. In order to obtain the likelihood in [2] for $\rho = 1$ (complete sampling), we must condition on $n$ lineages surviving to the present. Given that the initial birth event is fixed at time $t$ ago (or $T - t_2$ ago in the notation of Nee et al [1]), we divide $f_{\text{Nee}}$ by

$$(n-1)(P(0,t)(1-u_{(T-t_2)}))^2 u_{(T-t_2)}^{n-2}. \tag{44}$$

Here, we are conditioning that two lineages must survive to the present and that their combined number of descendants is $n$. The two lineages are independent, thus for any combination of numbers of progeny $(k, n-k)$ with $k > 0$ for the two lineages, we obtain $P(0,t)(1-u_{(T-t_2)})u_{(T-t_2)}^{k-1}P(0,t)(1-u_{(T-t_2)})u_{(T-t_2)}^{n-k-1} = (P(0,t)(1-u_{(T-t_2)}))^2 u_{(T-t_2)}^{n-2}$. There are $(n-1)$ such combinations. Division of $f_{\text{Nee}}$ by equation 44 gives

$$f_{\text{Y\&R}} := f(\mathbf{s}|n, F, \lambda, \mu, t)(n-2)!\lambda^{n-2} \prod_{j=3}^{n} \frac{(1-u_{(T-t_j)})P(t_j, T)}{u_{(T-t_2)}}. \tag{45}$$

This is $(n-2)!\lambda^{n-2} \prod_{j=1}^{n-2} \frac{p_1(s_j)}{u_{s_{n-1}}}$ in the notation of Thompson [19]. Letting time increase into the past, but indexing forwards and defining the deepest birth to have occurred at time $t_1$, we can obtain the likelihood of Yang and Rannala [2]. This change amounts to a relabelling of nodes in the Thompson notation $s_j \to t_{n-j}$:

$$f_{\text{Y\&R}} = (n-2)!\lambda^{n-2} \prod_{j=2}^{n-1} \frac{p_1(t_j)}{u_{t_1}}. \tag{46}$$

Noting that $u_t = 1 - P(0,t)\exp(-(\lambda-\mu)t)$, which is $\nu_t$ in Yang and Rannala [2],

$$f_{\text{Y\&R}} = (n-2)! \prod_{j=2}^{n-1} \lambda \frac{p_1(t_j)}{\nu_{t_1}}. \tag{47}$$

Finally, to obtain Gernhard's likelihood [20], $f_{\text{Gern}}$, we note that

$$u_t = \frac{\lambda}{\mu} \frac{\mu(1-\exp(-(\lambda-\mu)t))}{\lambda - \mu\exp(-(\lambda-\mu)t)} = \frac{\lambda}{\mu} p_0(t) \tag{48}$$

$$\Rightarrow \quad f_{\text{Y\&R}} = (n-2)! \prod_{j=2}^{n-1} \mu \frac{p_1(t_j)}{p_0(t_1)}. \tag{49}$$

Removing the ordering on the node times, and using the lemma [20] that any collection of unordered internal node times $\{s_2, s_3, \ldots, s_{n-1}\}$ is equally likely (and that there are $(n-2)!$ such orderings), we obtain $f_{\text{Gern}}$:

$$f_{\text{Gern}} = \prod_{j=2}^{n-1} \mu \frac{p_1(s_j)}{p_0(t_1)}. \tag{50}$$

Thus everything is nicely connected when we consider full sampling. To consider partial sampling lineages at the present, we must return to Kendall's derivations [3]. Nee et al. [1] looked to Kendall for their

derivation of $P_s(\tilde{t}, t)$. Analogous to derivations carried out in [1], a reconstructed sampled birth-death process can be shown to be equivalent to a pure birth process with variable rate $\lambda P_s(t, T)$. Conditioning in exactly the same way as the full sampling case yields $f_{\mathrm{Y\&R}}$ for $\rho \in (0, 1]$, which is also written in [21].

## S7 Derivation of surviving lineages through time within a deterministic model of transmission

Let $N(t)$ be the total number of infected individuals in the population, with $t$ measured backwards in time and initiated at the present. $M(t)$ is the number of individuals in the sampled subtree, where sampling only occurs at $t = 0$. Finally, $\tau(t)$ is the cumulative number of transmissions present in the sampled subtree in $[0, t]$.

$$\frac{dN}{dt} = \mu N - \lambda N, \tag{51}$$

$$\frac{dM}{dt} = -\lambda N \left(\frac{M}{N}\right)^2, \tag{52}$$

$$\frac{d\tau}{dt} = \lambda N \left(2\left(\frac{M}{N}\left(1 - \frac{M}{N}\right)\right)\frac{1}{2}\right) + \lambda N \left(\frac{M}{N}\right)^2 = \lambda M. \tag{53}$$

Note that as in [14,22], $N$ and $M$ are assumed to be large such that $M - 1 \approx M$ and $N - 1 \approx N$. Solving for $N(t)$ and $M(t)$, we obtain

$$N(t) = N(0)\exp((\mu - \lambda)t), \tag{54}$$

$$M(t) = \frac{(\mu - \lambda)\, N(0)}{\lambda + \frac{N(0)}{M(0)}\,(\mu - \lambda) - \lambda \exp(t(\lambda - \mu))}. \tag{55}$$

We wish to find what proportion of the total transmissions per lineage are unseen transmissions through time. Note that $\frac{d\tau}{dt}$ can be split into seen transmissions and unseen transmissions, and considering transmissions per lineage we divide through by $M(t)$. Thus, the rate of change of unseen transmissions

as a proportion of the total transmissions in a subtree is

$$1-\frac{M}{N}=1-\frac{(\mu-\lambda)}{\exp\left(-\left(\lambda-\mu\right)t\right)\left(\lambda+\frac{N(0)}{M(0)}\left(\mu-\lambda\right)\right)-\lambda} \tag{56}$$

$$=1-\frac{\frac{M(0)}{N(0)}\left(\lambda-\mu\right)}{\lambda\frac{M(0)}{N(0)}+\exp\left(-\left(\lambda-\mu\right)t\right)\left(\lambda\left(1-\frac{M(0)}{N(0)}\right)-\mu\right)}. \tag{57}$$

This is the same as $1-p_0(t)$ previously derived, the probability that a lineage sampled at time $t$ in the past survives into a sample at the present.

# References


1. Nee, S., May, R. M. & Harvey, P. H. 1994 The reconstructed evolutionary process. *Philosophical Transactions of the Royal Society of London. Series B: Biological Sciences*, **344**, 305-311. (doi:10.1098/rstb.1994.0068)

2. Yang, Z. & Rannala, B. 1997 Bayesian phylogenetic inference using DNA sequences: a Markov Chain Monte Carlo Method. *Molecular Biology and Evolution*, **14**, 717-724.

3. Kendall, D. G., 1948 On the generalized "birth-and-death" process. *The Annals of Mathematical Statistics*, **19**, 1-15.

4. Fagard, C. et al. 2003 A prospective trial of structured treatment interruptions in human immunodeficiency virus infection. *Archives of internal medicine*, **163**, 1220-1226. (doi:10.1001/archinte.163.10.1220)

5. Frater, A. J. et al. 2006 Passive sexual transmission of human immunodeficiency virus type 1 variants and adaptation in new hosts. *J. Virol.*, **80**, 7226-7234. (doi:10.1128/JVI.02014-05)

6. Los Alamos HIV sequence database. `http://www.hiv.lanl.gov/`.

7. Gaschen, B., Kuiken, C., Korber, B. & Foley, B. 2001 Retrieval and on-the-fly alignment of sequence fragments from the HIV database. *Bioinformatics (Oxford, England)*, **17**, 415-418.

8. Recombinant Identification Program. `http://www.hiv.lanl.gov/content/sequence/RIP/RIP.html`.

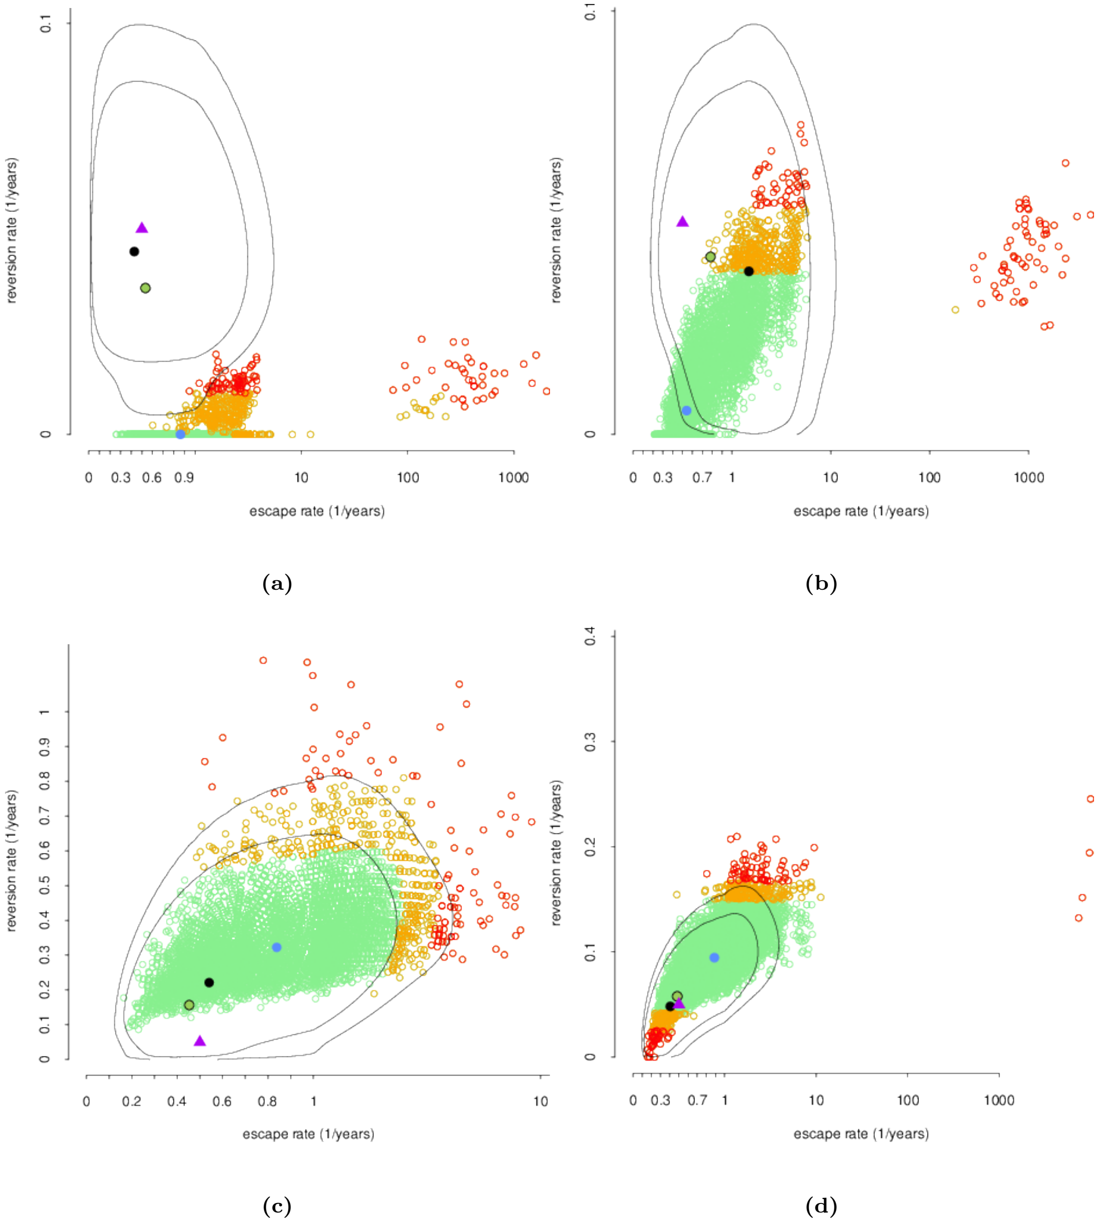


**Figure S1.** Four simulations with fixed escape and reversion parameters. In each, a birth-death tree with $(\lambda_{\text{esc}}, \lambda_{\text{rev}}) = (0.5, 0.05)$ $years^{-1}$. 10,000 bootstraps of the ODE approach are applied and shown as dots. These dots are coloured according to Mahalanobis distance (the top 1% and $1-5\%$ are coloured red and orange respectively, and the remainder green - see methods). Credible regions for the integrated method are shown in black. The MAP estimate in each case is shown as a black dot, and the truth as a purple triangle. The MAP for the true tree is the green outlined dot, and the ODE point estimate is the blue dot.

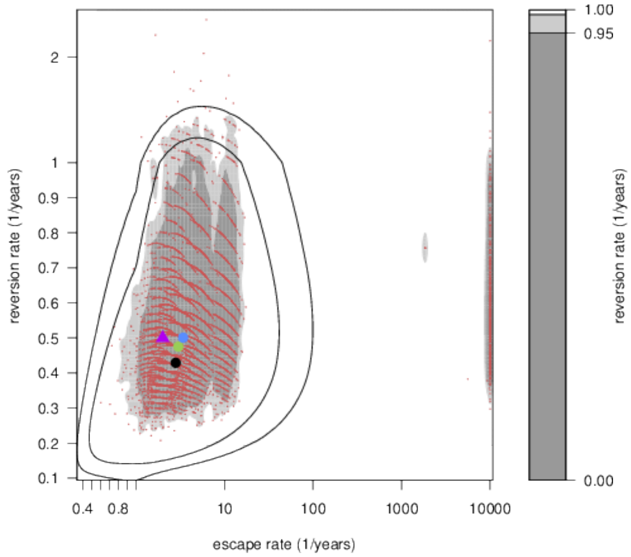


**(a)**

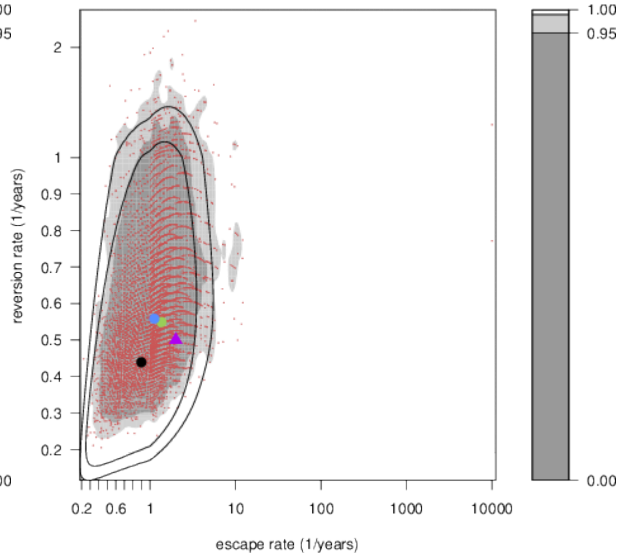


**(b)**

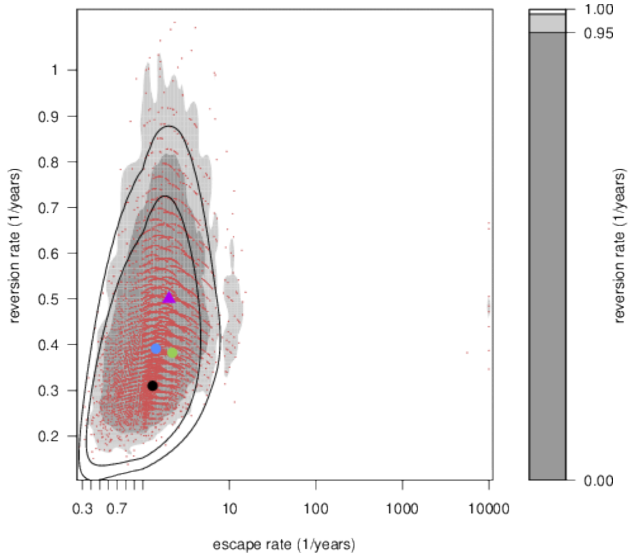


**(c)**

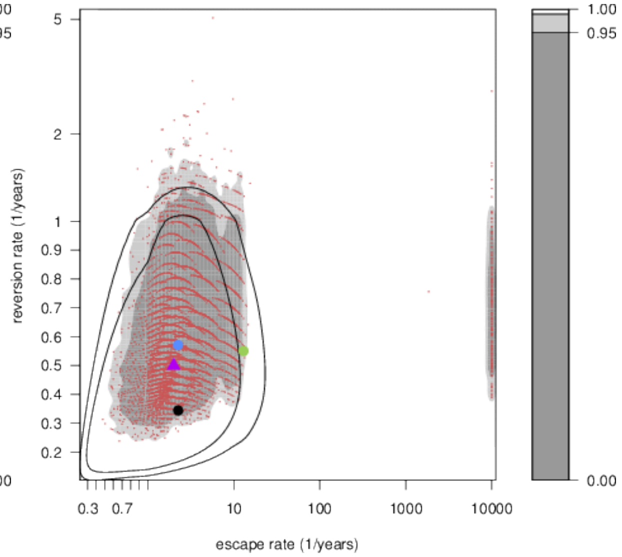


**(d)**

**Figure S2.** Four simulations with fixed escape and reversion parameters. True underlying rate $(\lambda_{\text{esc}}, \lambda_{\text{rev}}) = (2, 0.5)$ $years^{-1}$. 95% and 99% credible regions are shown in black. 10,000 ODE point estimates are shown in red, and contours coloured using a 2D kernel density estimate [23, 24] according to the key. The true rates are shown as a purple triangle, the MAP estimate is shown in black, and ODE point estimate in blue. The MAP based on the true underlying transmission tree is shown as a green outlined dot.

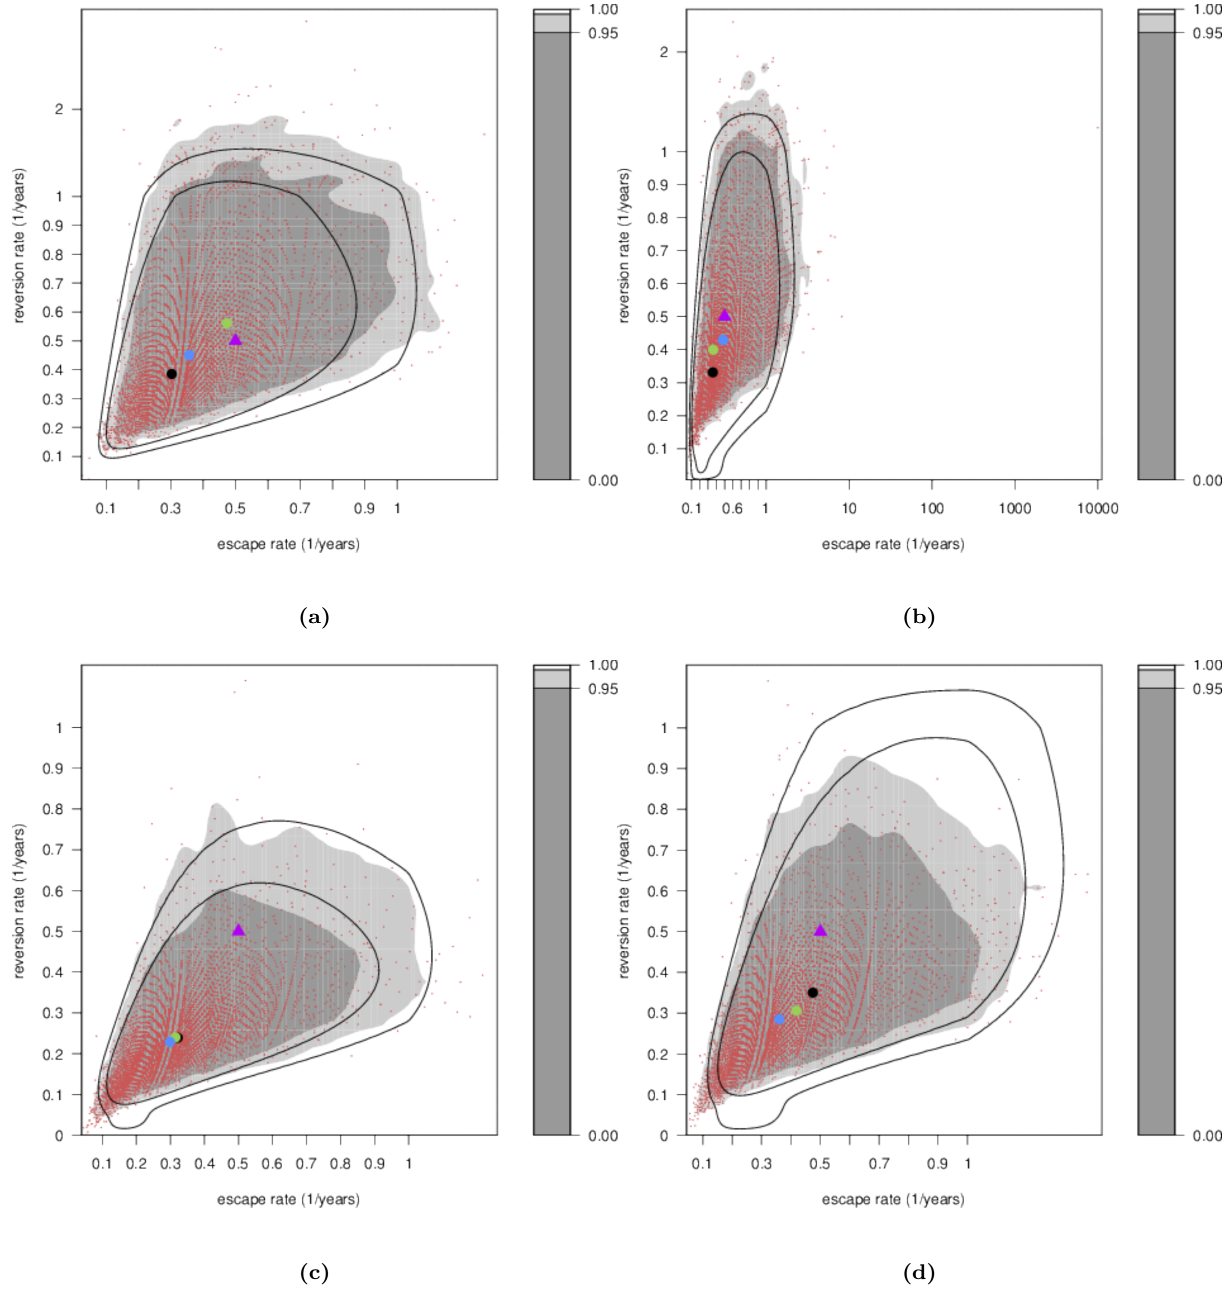


**Figure S3.** $(\lambda_{\rm esc}, \lambda_{\rm rev}) = (0.5, 0.5)\ years^{-1}$

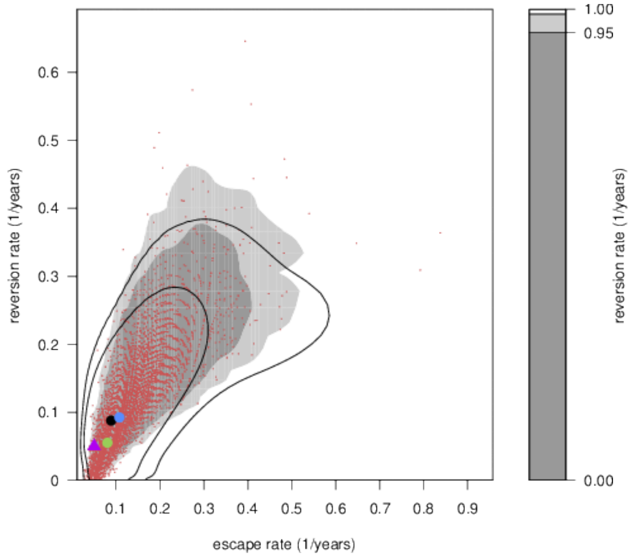


**(a)**

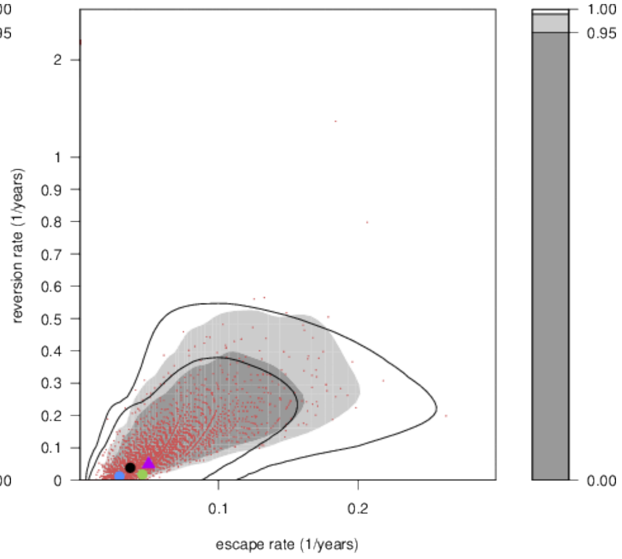


**(b)**

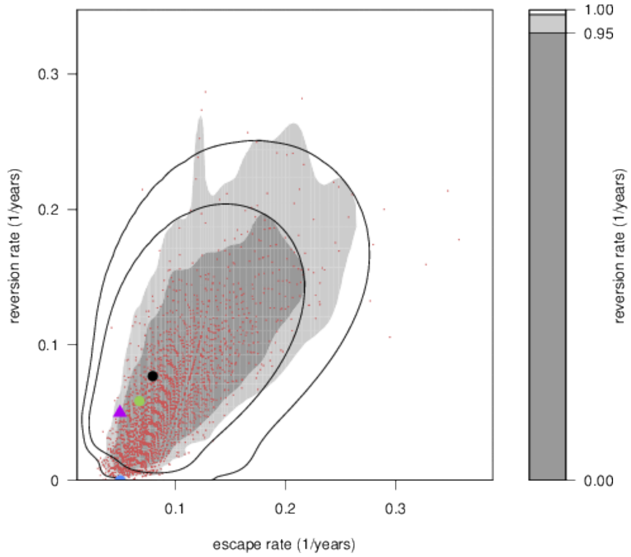


**(c)**

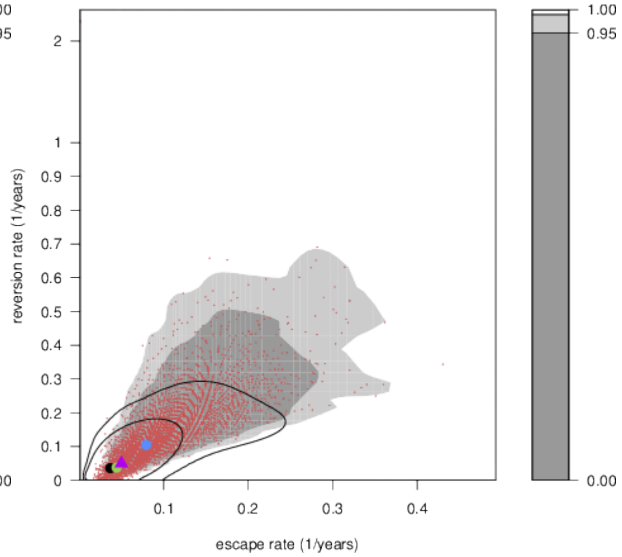


**(d)**

**Figure S4.** $(\lambda_{\text{esc}}, \lambda_{\text{rev}}) = (0.05, 0.05)$ $years^{-1}$

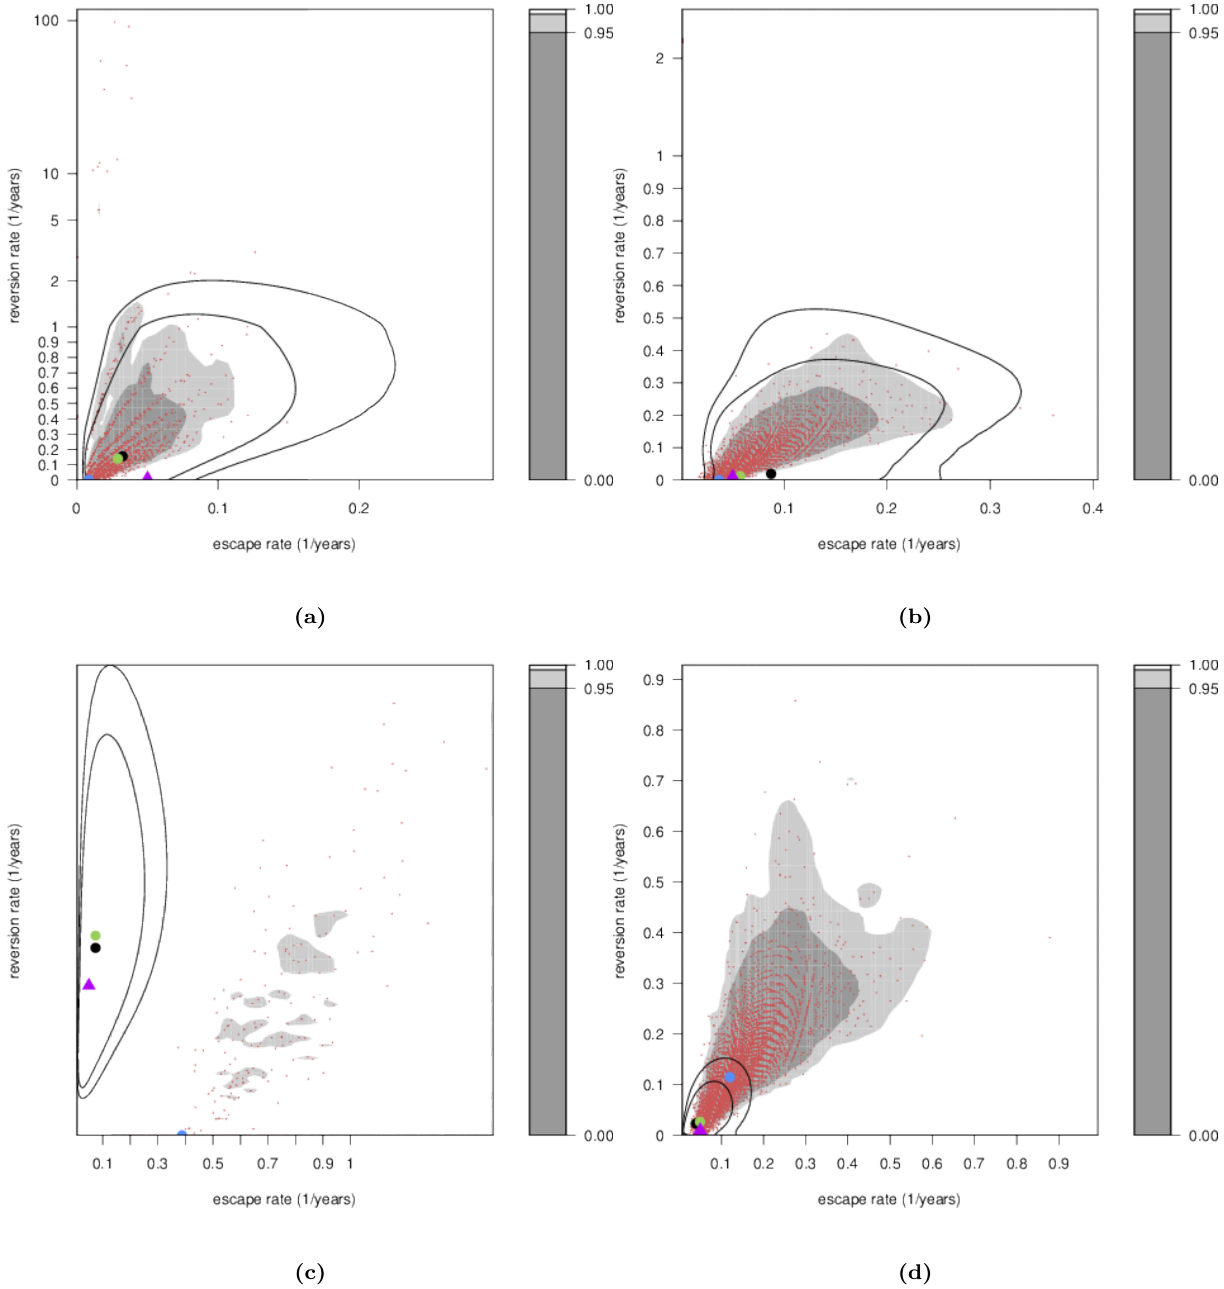


**Figure S5.** $(\lambda_{\text{esc}}, \lambda_{\text{rev}}) = (0.05, 0.01)$ $years^{-1}$

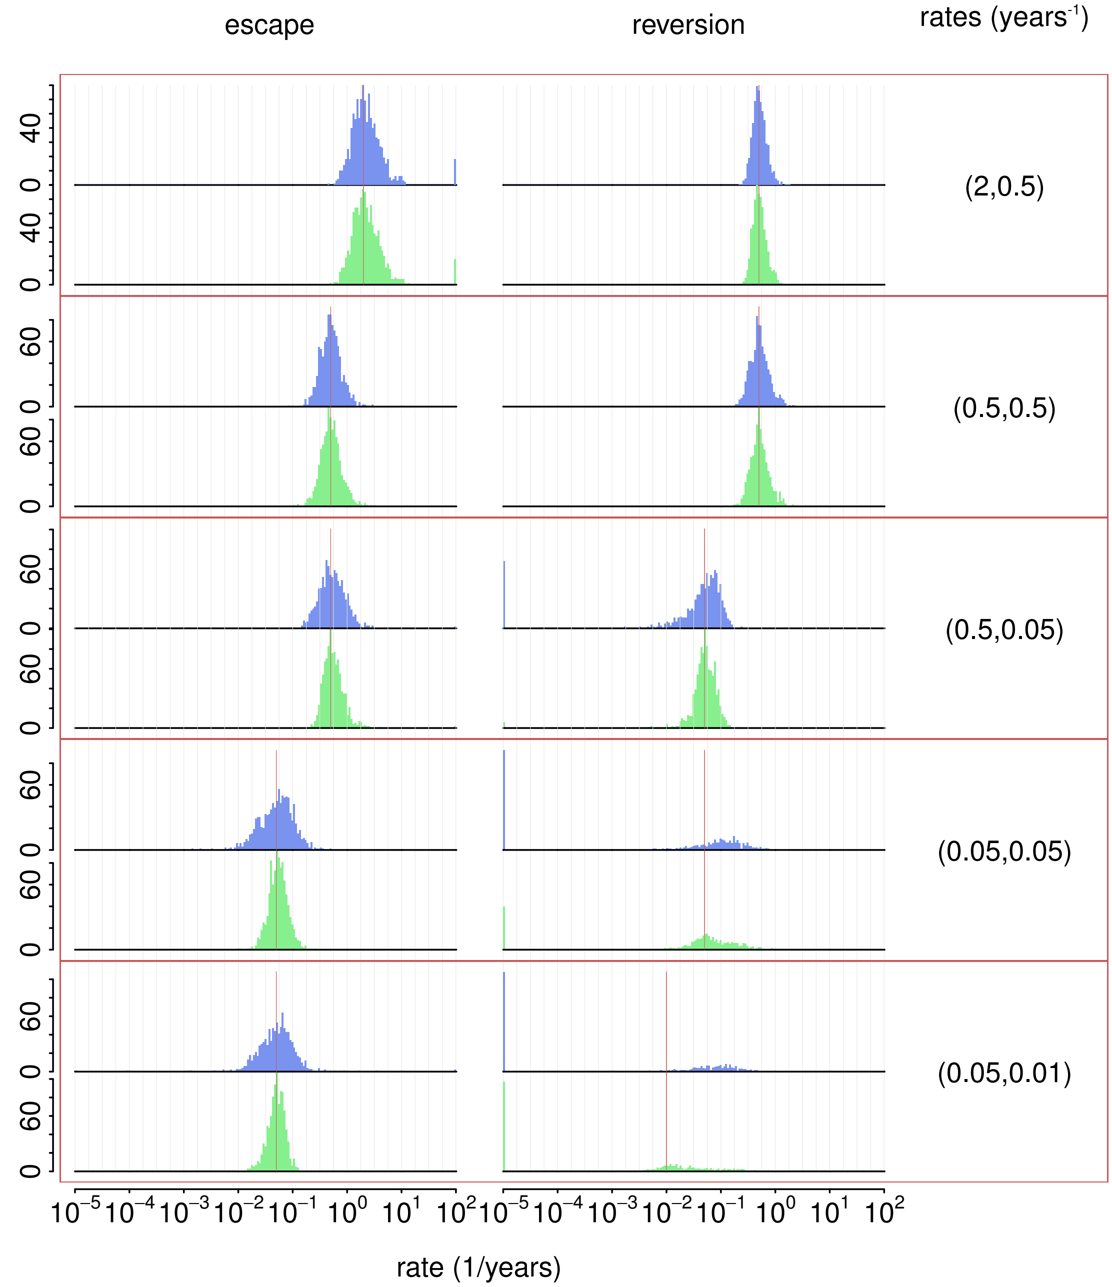


**Figure S6.** Histograms of MAPs using tree pruning and ODE point estimates for 5 parameter sets, $(\lambda_{\text{esc}}, \lambda_{\text{rev}}) = \{(2, 0.5), (0.5, 0.5), (0.5, 0.05), (0.05, 0.05), (0.05, 0.01)\}$ respectively. True rates for each parameter decrease down the figure. Histograms of the ODE point estimates are in blue, histograms of the MAP under tree pruning are in green. Rates $< 10^{-5}$ and $> 10^{2}$ are grouped in the histograms. In each plot, the truth is plotted in red.

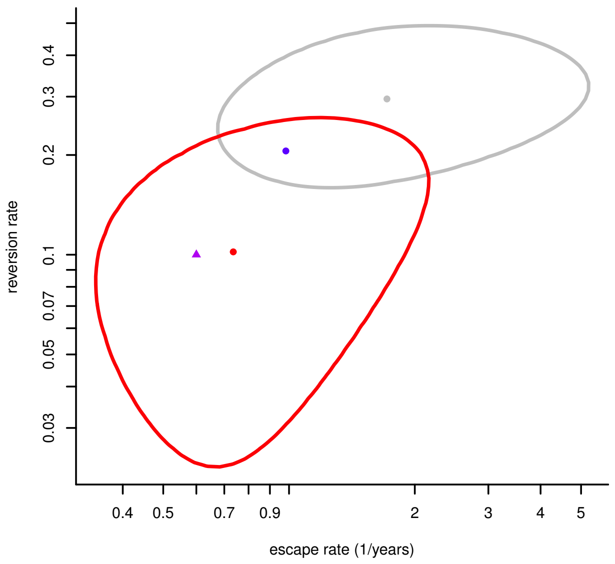


**Figure S7.** The true underlying sampled birth-death tree is shuffled 250 times, and our pruning algorithm applied, leading to the 90% credible region shown in grey, with MAP shown as a grey dot. The red credible region is the result of applying tree pruning to the true tip labellings. The purple triangle is the truth (0.6,0.1) and the blue dot is the point estimate from the ODE method.

9. Posada, D. 2008 jModelTest: phylogenetic model averaging. *Molecular Biology and Evolution*, **25**, 1253-1256. (doi:10.1093/molbev/msn083)

10. Drummond, A. J., Suchard, M. A., Xie, D. & Rambaut, A. 2012 Bayesian phylogenetics with BEAUti and the BEAST 1.7. *Molecular Biology and Evolution*, **29**, 1969-1973. (doi:10.1093/molbev/mss075)

11. Felsenstein, J. 1981 Evolutionary trees from DNA sequences: a maximum likelihood approach. *Journal of molecular evolution*, **17**, 368-376.

12. Cromer, D., Wolinsky, S. M. & McLean, A. R. 2010 How fast could HIV change gene frequencies in the human population? *Proceedings of the Royal Society B: Biological Sciences*, **277**, 1981-1989. (doi:10.1098/rspb.2009.2073)

13. Fryer, H. R., Frater, A. J., Duda, A., Roberts, M. G., Phillips, R. E., McLean, A. R., and The SPARTAC Trial Investigators. 2010 Modelling the evolution and spread of HIV immune escape mutants. *PLoS Pathog*, **6**, e1001196+. (doi:10.1371/journal.ppat.1001196)

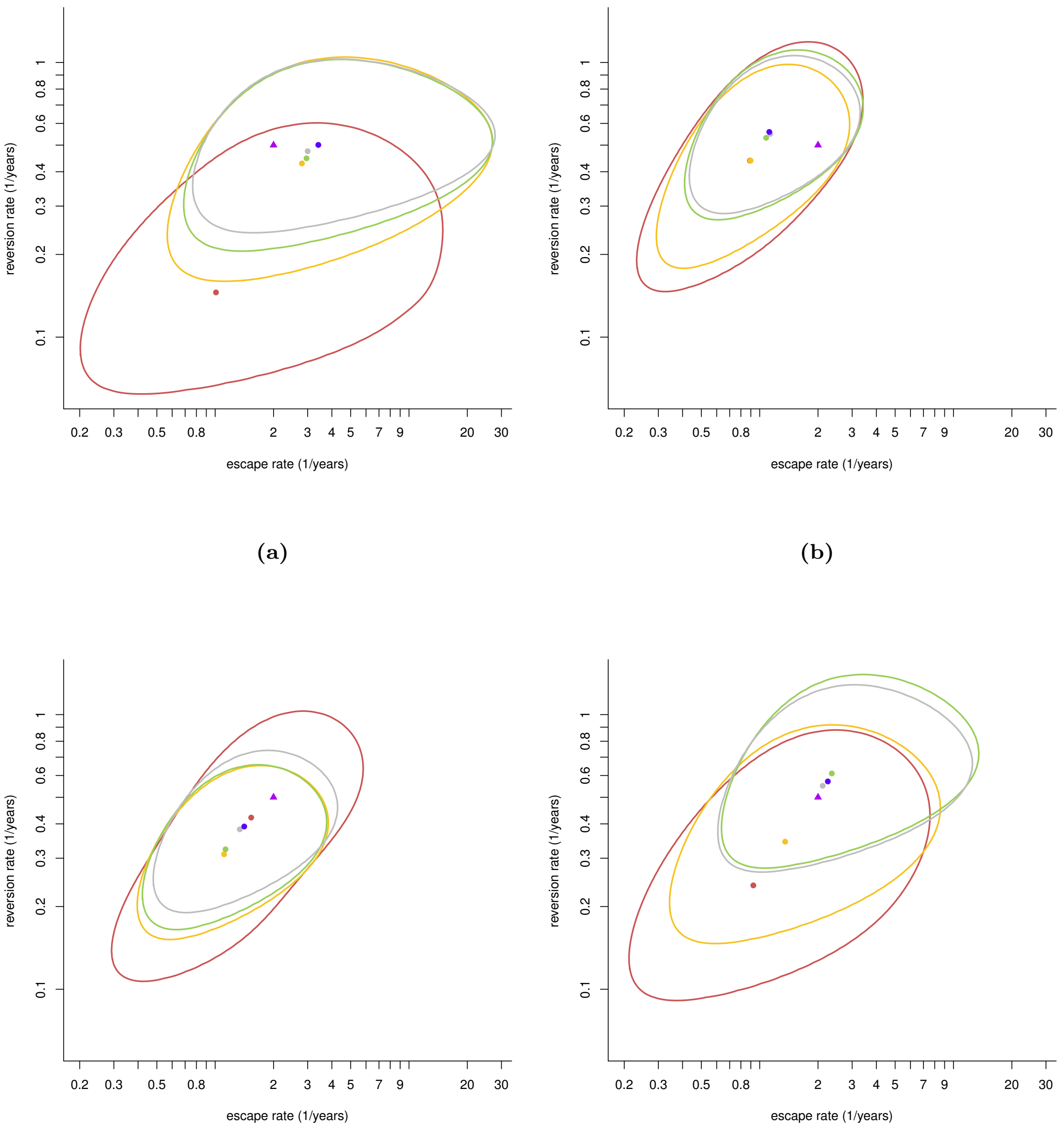


(a) (b)

(c) (d)

**Figure S8.** Four instances of simulations with reduced and accelerated substitution rates. In each, a 90% credible region is drawn for substitution rates at 0.2, 1 and 5 times the average of BEAST output for the SSITT gag sequence data under the $GTR + \Gamma + I$ model. Regions are coloured red, orange and green respectively. The truth, $(\lambda_{\text{esc}}, \lambda_{\text{rev}}) = (2, 0.5)$ $years^{-1}$ is shown as a purple triangle and MAPs for the corresponding credible regions are shown in the same colour. The ODE point estimate is displayed in blue in each simulation. Note the strong agreement between the ODE point estimate and MAP under these high $(\lambda_{\text{esc}}, \lambda_{\text{rev}})$ rates.

14. Frost, S. D. W & Volz, E. M. 2010 Viral phylodynamics and the search for an effective number of infections. *Philosophical Transactions of the Royal Society B: Biological Sciences*, **365**, 1879-1890. (doi:10.1098/rstb.2010.0060)

15. Morgan, D., Mahe, C., Mayanja, B., Okongo, M., Lubega, R. & Whitworth, J. A. 2002 HIV-1 infection in rural Africa: is there a difference in median time to AIDS and survival compared with that in industrialized countries? *AIDS (London, England)*, **16**, 597-603.

16. Marsh, S. G. E., Parham, P. & Barber, L. D. 2000 *The HLA FactsBook*. Academic Press, 1st edition.

17. Ahnert, K. & Mulansky, M. 2011 Odeint - solving ordinary differential equations in C++. *AIP Conference Proceedings*, **1389**, 1586-1589. (doi:10.1063/1.3637934)

18. Mahalanobis, P. C. 1936 On the generalised distance in statistics. *Proceedings National Institute of Science, India*, **2**, 49-55.

19. Thompson, E. A. 1975 *Human evolutionary trees*. Cambridge University Press.

20. Gernhard, T. 2008 The conditioned reconstructed process. *Journal of Theoretical Biology*, **253**, 769-778. (doi:10.1016/j.jtbi.2008.04.005)

21. Tanja Stadler. 2009 On incomplete sampling under birth-death models and connections to the sampling-based coalescent. *Journal of theoretical biology*, **261**, 58-66. (doi:10.1016/j.jtbi.2009.07.018)

22. Volz, E. M., Kosakovsky Pond, S. L., Ward, M. J., Leigh Brown, A. J., & Frost, S. D. W. 2009 Phylodynamics of infectious disease epidemics. *Genetics*, **183**, 1421-1430. (doi:10.1534/genetics.109.106021)

23. Wand, M. P. Fast computation of multivariate kernel estimators. 1994 *Journal of Computational and Graphical Statistics*, **3**, 433-445. (doi:10.1080/10618600.1994.10474656)

24. Wand, M. P & Jones, M. C. 1994 *Kernel Smoothing (Chapman & Hall/CRC Monographs on Statistics & Applied Probability)*, 1st edn, Chapman and Hall/CRC.
